# Supplementary material for: Human-Usable Password Schemas: Beyond Information-Theoretic Security
Source: arXiv:1906.00029 source file (2019-05-31)
Supplement: Supplementary file 1 [file AppendixA.tex]

% Appendix A

\chapter{Appendix Title Here} % Main appendix title

\label{AppendixA} % For referencing this appendix elsewhere, use \ref{AppendixA}

Write your Appendix content here.
